# Supplementary material for: IMTalker: Efficient Audio-driven Talking Face Generation with Implicit Motion Transfer
Source: arXiv:2511.22167 source file (2025-11-27)
Supplement: Supplementary file 1 [file X_suppl.tex]

% ==============================================
% Supplementary Material Start
% ==============================================

% 1. 这里的命令保留 (用于重置页码和生成标题)
\clearpage
\setcounter{page}{1}
\maketitlesupplementary
\appendix
% 2. 下面直接开始写具体的补充材料内容 (替换掉原本的 Rationale)

\section{Overview}
This supplementary material provides additional details and results to support the main paper. We organize the content as follows:
\begin{itemize}
    \item \textbf{Section \ref{sec:data}}: Dataset Composition and Processing
    \item \textbf{Section \ref{sec:arch}}: Model Architecture 
    \item \textbf{Section \ref{sec:objectives_metrics}}: Training Objectives and Metrics
    \item \textbf{Section \ref{sec:user_study}}: User Study
    \item \textbf{Section \ref{sec:addition}}: Additional Results
    \item \textbf{Section \ref{sec:demos}}: Qualitative Demonstrations
    \item \textbf{Section \ref{sec:limitations}}: Limitations and Ethical Considerations
\end{itemize}

% ==========================================
% Section 1: Data
% ==========================================
\section{Dataset Composition and Processing}
\label{sec:data}

\subsection{Dataset Composition}

Our training dataset is constructed from three publicly available benchmarks, primarily consisting of in-the-wild videos of interviews and speeches. These datasets encompass a wide range of subjects across different ages, genders, and ethnicities, ensuring comprehensive diversity for model generalization. The specific details of each dataset are as follows:

\begin{itemize}
    \item \textbf{VFHQ~\cite{xie2022vfhq}:} Originally collected for face super-resolution tasks, this dataset features high visual resolution. However, due to the absence of audio tracks, it is utilized exclusively for the training of the Renderer. After filtering, the dataset comprises approximately 33 hours of footage across 15,000 video clips.
    
    \item \textbf{VoxCeleb2~\cite{chung2018voxceleb2}:} This dataset consists primarily of a vast collection of English interview videos. It serves as the primary data source for training both the Renderer and the Motion Generator. After preprocessing and filtering, it yields approximately 256 hours of data across 160,339 video clips.
    
    \item \textbf{MultiTalk~\cite{sung2024multitalk}:} Featuring speakers from various countries speaking over 20 different languages, this dataset is employed solely for Renderer training to enhance the model's adaptability to diverse ethnic appearances and facial structures. Post-filtering, it contains 271 hours of footage comprising 183,935 videos.
\end{itemize}

Furthermore, to validate our method, we conduct qualitative and quantitative evaluations on randomly sampled subsets from the \textbf{HDTF \cite{zhang2021flow}}, \textbf{CelebV-Text \cite{yu2023celebv}}, \textbf{VFHQ \cite{xie2022vfhq}}, \textbf{RAVDESS \cite{livingstone2018ryerson}}, and \textbf{NeRSemble \cite{kirschstein2023nersemble}} datasets.

\subsection{Dataset Preprocessing}

To ensure high data quality and consistency across diverse sources, we implemented a rigorous data preprocessing and filtering pipeline prior to training. The specific steps are as follows:

\begin{enumerate}
    \item \textbf{Re-downloading Original Datasets:} To maximize video quality, we acquired the raw video data rather than using pre-processed versions. For \textbf{VoxCeleb2 \cite{chung2018voxceleb2}} and \textbf{MultiTalk \cite{sung2024multitalk}}, we re-downloaded the original videos using the URLs provided by the authors, discarding any clips with invalid or expired links. For \textbf{VFHQ \cite{xie2022vfhq}}, we utilized the officially released high-quality video files directly.
    
    \item \textbf{Face Alignment and Cropping:} We employed an off-the-shelf face tracker \cite{deng2019accurate} to detect facial landmarks for every frame. Based on these landmarks, we computed a stable, face-centric bounding box for each video sequence and performed cropping to isolate the facial region, ensuring consistent framing across the dataset.

    \item \textbf{Filtering and Standardization:} Following cropping, we applied a strict standardization and filtering protocol:
    \begin{itemize}
        \item \textbf{Format Normalization:} All video clips were resampled to a uniform frame rate of 25 fps and resized to a resolution of $512 ^ 2$. The corresponding audio tracks were resampled to 16 kHz.
        \item \textbf{Duration Constraints:} We filtered out clips shorter than 2 seconds to ensure sufficient temporal context and split clips longer than 10 seconds into shorter segments to facilitate efficient training.
        \item \textbf{Quality Control:} To maintain high visual fidelity, we excluded any raw videos with a resolution lower than $512 ^ 2$ pixels. Furthermore, to ensure data integrity, we removed samples with poor audio-visual synchronization based on low SyncNet \cite{prajwal2020lip} scores.
    \end{itemize}
\end{enumerate}

After applying this unified processing pipeline, we obtained the final training datasets described above. All test data used for evaluation underwent an identical preprocessing protocol to ensure consistency.

% ==========================================
% Section 2: Architecture
% ==========================================
\section{Model Architecture} \label{sec:arch}

In this section, we provide the detailed architectural configurations of our proposed IMTalker framework. The framework consists of two core components: Identity-Adaptive Motion Transfer Renderer and Flow-Matching Motion Generator.
\begin{table*}[t]
    \centering
    % 增加行高，提升可读性
    
    \caption{\textbf{Architecture details of the Generator.} The model integrates a frozen pre-trained Wav2Vec 2.0 encoder, condition projections, and a DiT backbone. $L$ denotes the sequence length of the aligned audio features and generated motion tokens. The reported parameter count excludes the pre-trained audio encoder.}
    \label{tab:model_arch}
    \resizebox{0.8\linewidth}{!}{ 
        \begin{tabular}{l l l c}
            \toprule
            \textbf{Module} & \textbf{Component} & \textbf{Configuration Details} & \textbf{Output Dim.} \\
            \midrule
            
            % --- Audio Encoder ---
            \textbf{Audio Encoder} & Wav2Vec 2.0 \footnotesize{(Frozen)} & 7 Conv Layers + 12 Transformer Layers & $L \times 768$ \\
            \midrule
            
            % --- Projections ---
            \multirow{3}{*}{\textbf{Projections}} 
             & Audio Proj. & \multirow{3}{*}{Linear $\to$ LayerNorm $\to$ SiLU} & \multirow{3}{*}{$L \times 32$} \\
             & Gaze Proj. & & \\
             & Pose/Cam Proj. & & \\
            \midrule
            
            % --- FMT Backbone ---
            \multirow{6}{*}{\textbf{DiT Backbone}} 
             & \multirow{2}{*}{Embeddings} & Time ($t$): MLP  & $512$ \\
             & & Input ($x$) / Cond ($c$): Linear  & $L \times 512$ \\
             \cmidrule(l{0.5em}r{0.5em}){2-4}
             
             & \multirow{3}{*}{Transformer Blocks} 
             & Depth: 8 Blocks & \multirow{3}{*}{$L \times 512$} \\
             & & Structure: Hidden=512 & \\
             & & Norm: AdaLN-Modulation & \\
             \cmidrule(l{0.5em}r{0.5em}){2-4}
             
             & Decoder Head & AdaLN $\to$ Linear & $L \times 32$ \\
            \midrule
            
        \end{tabular}
    }
\end{table*}
\begin{table*}[t]
    \centering
    % 增加行间距，提升可读性
    
    \caption{\textbf{Architecture Details of the Renderer.} The model employs a hybrid architecture. We detail the resolution changes (Res) alongside the channel dimensions ($C$). Note that the entire architecture is trained from scratch.}
    \label{tab:imt_renderer_arch}
    \resizebox{0.9\linewidth}{!}{
        \begin{tabular}{l l l c c}
            \toprule
            \textbf{Module} & \textbf{Sub-Module} & \textbf{Configuration / Structure} & \textbf{Res ($H{\times}W$)} & \textbf{Channels ($C$)} \\
            \midrule
            
            % --- Encoders ---
            \multirow{4}{*}{\textbf{Encoders}} 
             & Identity Enc. & 5$\times$ ResConvBlocks (Downsample) & $256^2 \to 8^2$ & $512$ \\
             \cmidrule(l{0.5em}r{0.5em}){2-5} % 细线分隔
             & \multirow{2}{*}{Motion Enc.} & 5$\times$ ResConvBlocks (Downsample) & $256^2 \to 8^2$ & $32$ (Latent) \\
             & & Head: Linear Projection & $8^2 \to 1^2$ & - \\
            \midrule
            
            % --- Adapter ---
            \textbf{Adapter} & Identity-Adaptive & MLP & $1^2 \to 1^2$ & $32 \to 32$ \\
            \midrule
            
            % --- Motion Transfer ---
            \multirow{4}{*}{\textbf{Motion Transfer}} 
             & Motion Dec. & StyleGAN-style Modulated Conv & $4^2 \to 64^2$ & $512 \to 128$ \\
             \cmidrule(l{0.5em}r{0.5em}){2-5}
             & \multirow{2}{*}{Cross Attn.} & Low-Res: Standard Attention & $8^2, \dots, 64^2$ & $512, \dots, 128$ \\
             & & High-Res: Guided Sparse Resampler & $128^2, 256^2$ & $64, 32$ \\
            \midrule

            % --- Synthesis Net ---
            \multirow{6}{*}{\textbf{Synthesis Net}} 
             & Backbone & 5$\times$ Up-sampling ResConvBlocks & $8^2 \to 256^2$ & $512 \to 32$ \\
             \cmidrule(l{0.5em}r{0.5em}){2-5}
             & \multirow{2}{*}{\shortstack[l]{Hybrid\\Transformer}} & Low-Res: Standard Transformer & $8^2, \dots, 64^2$ & $512, \dots, 128$ \\
             & & High-Res: Swin Transformer & $128^2, 256^2$ & $64, 32$ \\
             \cmidrule(l{0.5em}r{0.5em}){2-5}
             & \multirow{2}{*}{Output Head} & Conv2d ($32 \to 3$) & $256^2$ & \multirow{2}{*}{$3$ (RGB)} \\
             & & $\hookrightarrow$ PixelShuffle (UpScale $\times 2$) & $256^2 \to 512^2$ & \\
            \bottomrule
        \end{tabular}
    }
\end{table*}
\subsection{Identity-Adaptive Motion Transfer Renderer (Renderer)}
The Renderer encodes identity and motion features from input images to synthesize high-fidelity novel frames. As detailed in Table \ref{tab:imt_renderer_arch}, the architecture comprises two structurally similar CNN-based encoders: an Identity Encoder and a Motion Encoder. These are followed by a StyleGAN-style motion decoder for motion map generation and a motion transfer module based on standard attention. The final image generation is performed by a synthesis network that integrates Residual Convolutional Blocks (ResConvBlocks) with standard Transformer blocks (at lower resolutions) and Swin Transformer blocks (at higher resolutions). The total parameter count for the renderer is approximately 124.1 M. Notably, the entire model is trained from scratch without relying on any pre-trained modules.

\subsection{Flow-Matching Motion Generator (Generator)}
The Generator is responsible for predicting facial motion dynamics from audio signals. As detailed in Table \ref{tab:model_arch}, it employs a pre-trained Wav2Vec 2.0 \cite{baevski2020wav2vec} model to extract audio features. The core backbone is a DiT comprising 8 transformer blocks with a hidden dimension of 512. We utilize AdaLN-Modulation to inject timestep and condition embeddings. The total parameter count for this module is approximately 38.8 M, excluding the pre-trained Wav2Vec 2.0 \cite{baevski2020wav2vec} encoder.
\section{Training Objectives and Metrics}
\label{sec:objectives_metrics}

\subsection{Training Objectives}
As outlined in the main paper, for training the renderer, our total objective function is defined as a weighted sum of reconstruction, perceptual, adversarial, and distance losses:
\begin{equation}
    \mathcal{L}_{\text{total}} = \lambda_{\text{rec}}\mathcal{L}_{\text{rec}} + \lambda_{\text{lpips}}\mathcal{L}_{\text{lpips}} + \lambda_{\text{GAN}}\mathcal{L}_{\text{GAN}}  + \lambda_{\text{dist}}\mathcal{L}_{\text{dist}}.
\end{equation}
Empirically, we set the weights $\lambda_{\text{rec}}$, $\lambda_{\text{lpips}}$, $\lambda_{\text{GAN}}$, and $\lambda_{\text{dist}}$ to $1$, $10$, $0.2$, and $1$, respectively.

The detailed formulation for each component is as follows:

\begin{itemize}
    \item \textbf{Reconstruction Loss ($\mathcal{L}_{\text{rec}}$):} To enforce pixel-level consistency between the generated frame $\hat{I}$ and the ground-truth frame $I$, we employ the $L_1$ reconstruction loss. This term ensures the synthesis of sharp low-level details:
    \begin{equation}
        \mathcal{L}_{\text{rec}} = \| I - \hat{I} \|_1.
    \end{equation}

    \item \textbf{Perceptual Loss ($\mathcal{L}_{\text{lpips}}$):} To improve visual quality and capture high-frequency details that align with human perception, we utilize the Learned Perceptual Image Patch Similarity (LPIPS) loss. We extract feature maps $\phi_l(\cdot)$ from the $l$-th layer of a pre-trained VGG \cite{simonyan2014very} network:
    \begin{equation}
        \mathcal{L}_{\text{lpips}} = \sum_{l} \left\| \phi_l(I) - \phi_l(\hat{I}) \right\|_2.
    \end{equation}

    \item \textbf{Adversarial Loss ($\mathcal{L}_{\text{GAN}}$):} To ensure photorealism and mitigate blurry artifacts, we adopt an adversarial loss mechanism using a hinge loss \cite{lim2017geometric} formulation. The generator minimizes:
    \begin{equation}
        \mathcal{L}_{\text{GAN}} = - \mathbb{E}_{\hat{I}} [D(\hat{I})].
    \end{equation}
    The discriminator $D$ is optimized concurrently to minimize:
    \begin{equation}
        \mathcal{L}_{D} = \mathbb{E}_{I} [\text{ReLU}(1 - D(I))] + \mathbb{E}_{\hat{I}} [\text{ReLU}(1 + D(\hat{I}))].
    \end{equation}

    \item \textbf{Distance Loss ($\mathcal{L}_{\text{dist}}$):} This loss is designed to enhance the adaptability of motion across different identities. Specific details are elaborated in the main text.
\end{itemize}

For training the generator, we employ the standard Optimal Transport \cite{liu2022flow} flow matching loss, denoted as $\mathcal{L}_{\text{FM}}$ in the main text.

\subsection{Evaluation Metrics}
\label{sec:metrics_details}
We conduct a comprehensive evaluation using metrics covering image quality, identity preservation, motion accuracy, and lip-synchronization.

\begin{itemize}
    \item \textbf{PSNR (Peak Signal-to-Noise Ratio):} Measures the pixel-level reconstruction quality. Higher values indicate lower distortion compared to the ground truth.
    
    \item \textbf{SSIM (Structure Similarity Index Measure) \cite{wang2004image}:} Evaluates the structural similarity (luminance, contrast, and structure) between the generated and real images.
    
    \item \textbf{LPIPS (Learned Perceptual Image Patch Similarity) \cite{zhang2018unreasonable}:} Computes the distance between image patches in deep feature space (using AlexNet \cite{krizhevsky2012imagenet}), aligning better with human perceptual judgment than PSNR/SSIM. Lower values indicate better perceptual quality.
    
    \item \textbf{FID (Fréchet Inception Distance) \cite{heusel2017gans}:} Measures the distance between the distributions of synthesized and real images in the feature space of an Inception-v3 \cite{szegedy2016rethinking} network. Lower FID indicates more realistic individual frames.
    
    \item \textbf{FVD (Fréchet Video Distance) \cite{unterthiner2018towards}:} An extension of FID for video, assessing the temporal coherence and quality of the generated video sequences. We use StyleGAN-V \cite{skorokhodov2022stylegan} as our feature extractor, capturing spatiotemporal features using a sliding window of 25 consecutive frames.
    
    \item \textbf{CSIM (Cosine Similarity of Identity Embedding) \cite{deng2019arcface}:} Evaluates identity preservation by calculating the cosine similarity between the identity embeddings of the generated frames and the source subject, extracted using a pretrained ArcFace \cite{deng2019arcface} network. Higher values indicate better identity retention.
    
    \item \textbf{AED (Average Expression Distance) \cite{retsinas2024smirk}:} Quantifies the fidelity of expression reenactment. It computes the average $L_2$ distance between the expression parameters of the generated frames and the ground truth, extracted via the SMIRK \cite{retsinas2024smirk} estimator. Lower values imply more accurate expression transfer.
    
    \item \textbf{APD (Average Pose Distance) \cite{retsinas2024smirk}:} Assesses the accuracy of head pose control. It calculates the average $L_2$ distance between the estimated 6-DoF head pose angles of the generated video and the driving signal, extracted via the SMIRK \cite{retsinas2024smirk} estimator. Lower values indicate better pose alignment.
    
    \item \textbf{MAE (Mean Angular Error) \cite{abdelrahman2023l2cs}:} Evaluates the accuracy of eye gaze direction. It measures the mean angular $L_2$ error between the gaze vectors of the generated faces and the ground truth, using the L2CS-Net \cite{abdelrahman2023l2cs} estimator. Lower values signify more precise gaze direction.
    
    \item \textbf{Sync-C (Lip-Sync Error Confidence) \cite{prajwal2020lip}:} Measures the confidence score of the audio-visual synchronization using the pre-trained SyncNet \cite{Chung16a} model. Higher values indicate better lip-sync quality and stronger correlation between lip movements and the audio track.
    
    \item \textbf{Sync-D (Lip-Sync Error Distance) \cite{prajwal2020lip}:} Represents the audio-visual distance computed by SyncNet \cite{Chung16a}. It measures the feature distance between the audio track and the visual lip movements. Lower values indicate more precise synchronization.
\end{itemize}
\begin{table}[t]
    \centering
    % --- 子表 (a): IA 消融 ---
    \begin{subtable}{\linewidth}
        \centering
        \resizebox{\linewidth}{!}{%
            \begin{tabular}{lccccc}
                \toprule
                Method & FID$\downarrow$ & CSIM$\uparrow$ & AED$\downarrow$ & APD$\downarrow$ & MAE$\downarrow$ \\
                \midrule
                w/o IA & 55.685 & 0.741 & \textbf{0.562} & 0.025 & 7.681 \\
                w/ IA  & \textbf{53.137} & \textbf{0.824} & 0.581 & \textbf{0.024} & \textbf{7.553} \\
                \bottomrule
            \end{tabular}%
        }
        \caption{Ablation study on the Identity-Adaptive (IA) Module.}
        \label{tab:ablation_ia}
    \end{subtable}
    
    \vspace{8pt} % 两个子表之间的间距

    % --- 子表 (b): Fine-tuning 消融 ---
    \begin{subtable}{\linewidth}
        \centering
        \resizebox{\linewidth}{!}{%
            \begin{tabular}{lccccc}
                \toprule
                Method & PSNR$\uparrow$ & SSIM$\uparrow$ & LPIPS$\downarrow$ & CSIM$\uparrow$ & FID$\downarrow$ \\
                \midrule
                w/o HA & 27.581 & 0.883 & 0.045 & 0.894 & 8.539 \\
                w/ HA  & \textbf{28.458} & \textbf{0.899} & \textbf{0.037} & \textbf{0.898} & \textbf{7.426} \\
                \bottomrule
            \end{tabular}%
        }
        \caption{Ablation study on the Hybrid Attention (HA) Strategy.}
        \label{tab:ablation_ha}
    \end{subtable}
    
    \caption{\textbf{Ablation Studies.} We evaluate the impact of (a) the  Identity-Adaptive (IA) Module and (b) the Hybrid Attention (HA) Strategy on model performance.}
    \label{tab:ablation_combined}
\end{table}
\begin{table}[t]
    \centering
    \caption{\textbf{Impact of Motion Latent Dimension.} Quantitative results under self-driven and cross-driven settings with different motion latent Dimension.}
    \resizebox{\linewidth}{!}{%
        \begin{tabular}{lccccc}
            \toprule
            & \multicolumn{3}{c}{Self-driven} & \multicolumn{2}{c}{Cross-driven} \\
            \cmidrule(lr){2-4} \cmidrule(lr){5-6}
            Dim & PSNR$\uparrow$ & SSIM$\uparrow$ & LPIPS$\downarrow$ & AED$\downarrow$ & CSIM$\uparrow$ \\
            \midrule
            16  & 28.193 & 0.895 & 0.043 & 0.596 & 0.823 \\
            32  & 28.458 & 0.899 & 0.037 & \textbf{0.581} & \textbf{0.824} \\
            128 & 28.561 & 0.902 & 0.034 & 0.587 & 0.816 \\
            512 & \textbf{28.599} & \textbf{0.903} & \textbf{0.033} & 0.594 & 0.811 \\
            \bottomrule
        \end{tabular}%
    }
    \label{tab:dimension_ablation}
\end{table}
\begin{figure}[t]
    \centering
    % 调整子图之间的间距，使其尽可能紧凑
    \setlength{\tabcolsep}{0.5pt} 
    
    % 定义单个图片的宽度：
    % 单栏宽度下，4张图并排，0.245 是极限宽度(留微小缝隙)
    \newcommand{\cols}{0.245\linewidth}

    % --- 第一行: video_01 ---
    % 注意：行尾加 % 是为了防止产生多余空格导致换行
    \begin{subfigure}{\cols}
        \includegraphics[width=\linewidth]{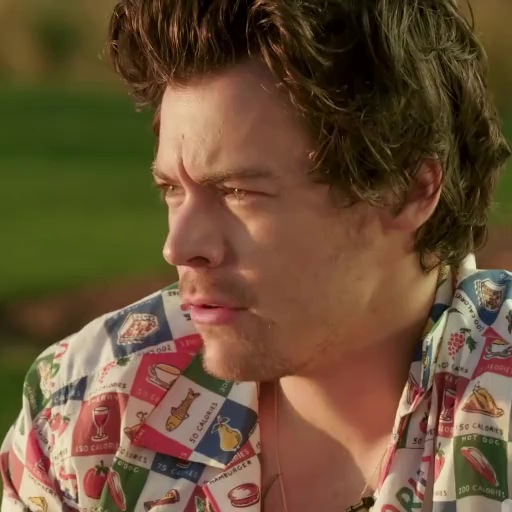}
    \end{subfigure}\hfill%
    \begin{subfigure}{\cols}
        \includegraphics[width=\linewidth]{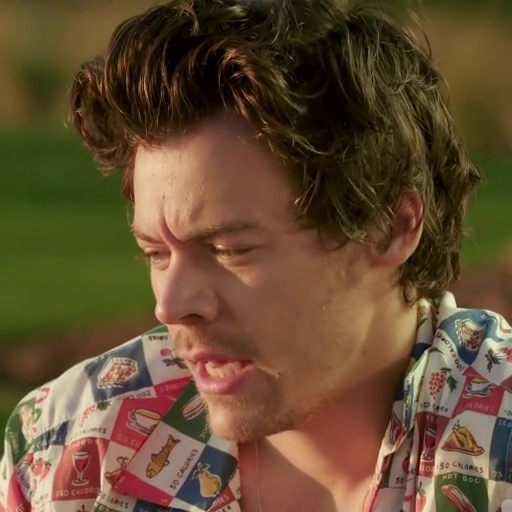}
    \end{subfigure}\hfill%
    \begin{subfigure}{\cols}
        \includegraphics[width=\linewidth]{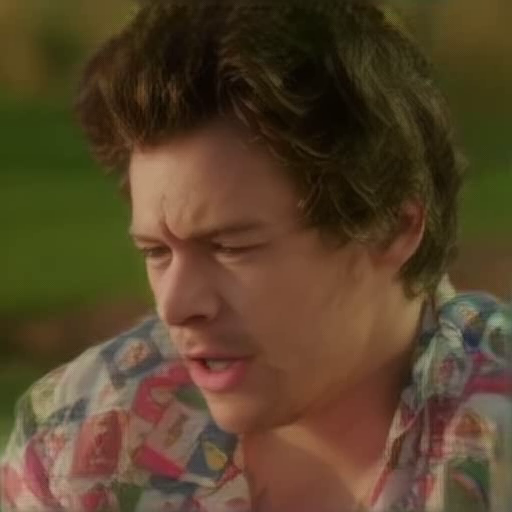}
    \end{subfigure}\hfill%
    \begin{subfigure}{\cols}
        \includegraphics[width=\linewidth]{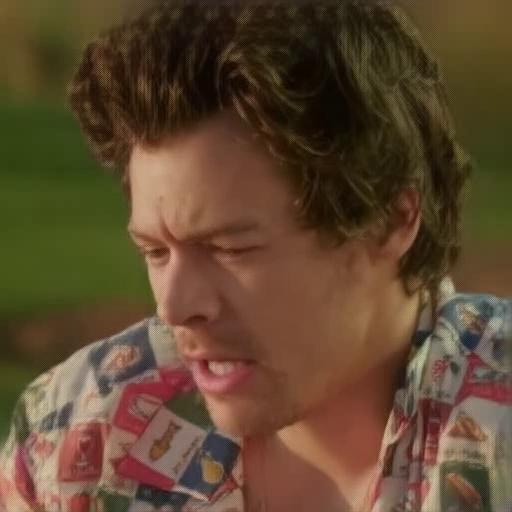}
    \end{subfigure}

    \vspace{1pt} % 行间微小垂直间距

    % --- 第二行: video_02 (带底部标注) ---
    \begin{subfigure}{\cols}
        \includegraphics[width=\linewidth]{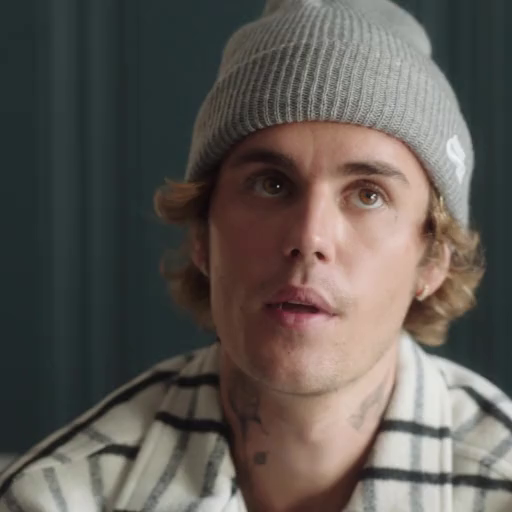}
        % caption* 不显示 (a), (b) 编号，只显示文字
        \caption*{Source} 
    \end{subfigure}\hfill%
    \begin{subfigure}{\cols}
        \includegraphics[width=\linewidth]{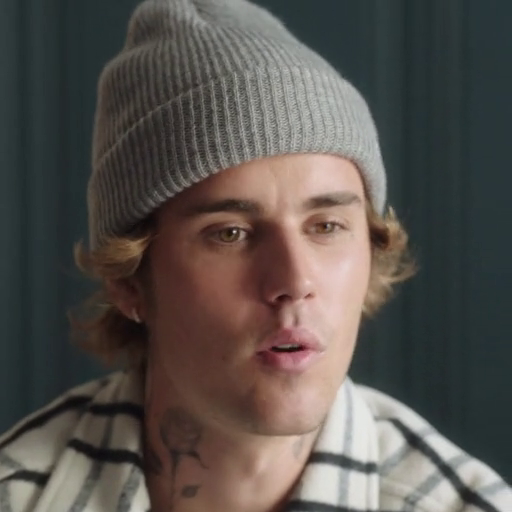}
        \caption*{Driving}
    \end{subfigure}\hfill%
    \begin{subfigure}{\cols}
        \includegraphics[width=\linewidth]{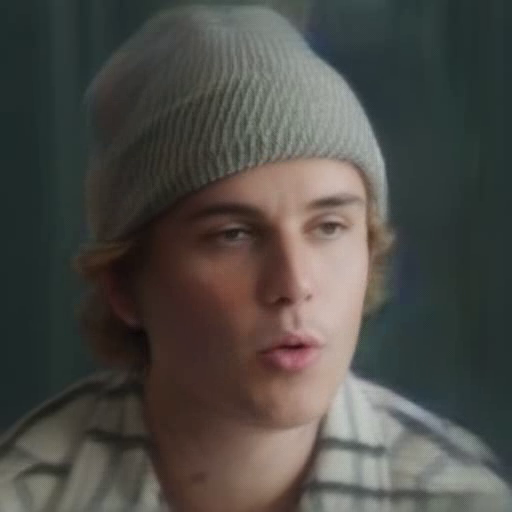}
        \caption*{w/o HA}
    \end{subfigure}\hfill%
    \begin{subfigure}{\cols}
        \includegraphics[width=\linewidth]{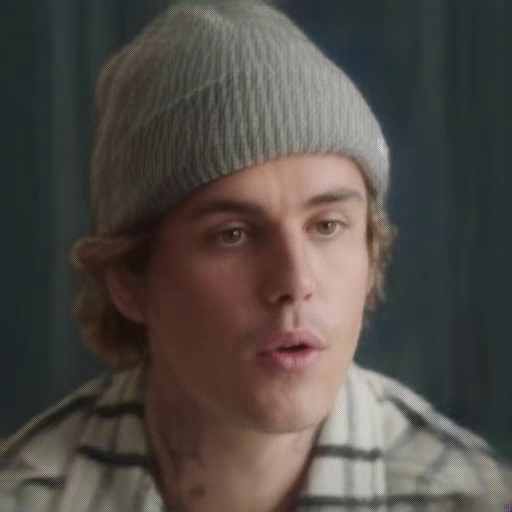}
        \caption*{w/ HA}
    \end{subfigure}

    % --- 图注 ---
    \vspace{-5pt} % 向上拉近图注与图片的距离，节省空间
    \caption{Visual comparison}
    \label{fig:ha_qualitative}
\end{figure}
\section{Additional Results}
\label{sec:addition}

In this section, we provide comprehensive quantitative and qualitative analyses to further validate the effectiveness of our proposed modules and parameter choices.

\subsection{Ablation on Identity-Adaptive (IA) Module}
In the main manuscript, we presented qualitative comparisons demonstrating the efficacy of the Identity-Adaptive (IA) module. To further substantiate these findings, we provide quantitative evaluations in Table \ref{tab:ablation_combined} (a), conducted on the HDTF \cite{zhang2021flow} dataset under a cross-driven setting. The results clearly indicate that the IA module enhances the accuracy of motion transfer. Most notably, it significantly improves identity preservation during the cross-identity motion transfer process, effectively preventing identity leakage from the driving source.

\subsection{Ablation on Hybrid Attention (HA) Strategy}
As discussed in the main paper, we employ a hierarchical coarse-to-fine guided attention strategy (Hybrid Attention, HA) to obtain high-resolution aligned feature maps $F_{\text{aligned, fine}}$. This strategy replaces full attention mechanisms at high resolutions, thereby significantly reducing the computational burden. To validate its effectiveness, we conducted ablation studies comparing a baseline configuration that applies cross-attention exclusively at low resolutions (denoted as w/o HA) against our proposed strategy, which integrates joint processing at both low and high resolutions (w/ HA).
Table \ref{tab:ablation_combined} (b) presents the quantitative results on the HDTF \cite{zhang2021flow} dataset. The data demonstrates that the HA strategy enhances the visual quality of self-reconstruction, contributing to the generation of sharper and higher-quality videos. Furthermore, as shown in Figure \ref{fig:ha_qualitative}, qualitative comparisons reveal that the HA strategy not only improves identity preservation but also facilitates the reconstruction of fine-grained facial motions.

\subsection{Analysis of Motion Latent Dimension}
We conducted experiments to analyze the impact of varying motion Latent dimensions on model performance. As illustrated in Table \ref{tab:dimension_ablation}, increasing the motion latent dimension leads to higher scores in self-reenactment benchmarks, indicating superior reconstruction capabilities. However, in the cross-reenactment setting, we observe a degradation in both motion transfer accuracy and identity preservation as the dimensions increase. Additionally, higher dimensions resulted in slower convergence rates during the training of the Generator. Balancing the requirements of both video-driven and audio-driven tasks, we selected 32 as the default dimension for our model to ensure optimal performance and efficiency.
% Section 4: User Study
% ==========================================
\section{User Study} \label{sec:user_study}
% Table 1: Video-driven
\begin{table*}[t]
    \centering
    \small % Use small font for better fit
    \setlength{\tabcolsep}{3.5pt} % Adjust column spacing
    \caption{\textbf{User Study on Video-driven Generation.} We report the Mean $\pm$ Variance (1-5 scale). The best results are \textbf{bolded} and the second best are \underline{underlined}. IMTalker achieves the best performance across all metrics.}
    \label{tab:user_study_video}
    \begin{tabular}{lcccccc}
        \toprule
        \textbf{Metric} & EDTalk \cite{tan2024edtalk} & LIA \cite{wang2022latent} & LivePortrait \cite{guo2024liveportrait} & MCNet \cite{hong2023implicit} & X-Portrait \cite{xie2024x}& \textbf{IMTalker (Ours)} \\
        \midrule
        Visual Quality & 3.50 $\pm$ 1.20 & \underline{3.77 $\pm$ 0.86} & 3.70 $\pm$ 0.93 & 3.44 $\pm$ 1.17 & 3.21 $\pm$ 1.57 & \textbf{4.08 $\pm$ 0.89} \\
        Motion Accuracy & 3.60 $\pm$ 1.03 & \underline{3.63 $\pm$ 0.97} & 3.59 $\pm$ 1.08 & 3.44 $\pm$ 1.21 & 3.14 $\pm$ 1.57 & \textbf{4.28 $\pm$ 0.74} \\
        ID Consistency & 3.60 $\pm$ 1.25 & \underline{3.78 $\pm$ 1.18} & 3.68 $\pm$ 1.05 & 3.64 $\pm$ 1.29 & 3.13 $\pm$ 1.30 & \textbf{3.98 $\pm$ 1.09} \\
        \bottomrule
    \end{tabular}
\end{table*}

% Table 2: Audio-driven
\begin{table*}[t]
    \centering
    \small
    \setlength{\tabcolsep}{3.8pt}
    \caption{\textbf{User Study on Audio-driven Generation.} We report the Mean $\pm$ Variance (1-5 scale). The best results are \textbf{bolded} and the second best are \underline{underlined}. IMTalker achieves the best performance across all metrics.}
    \label{tab:user_study_audio}
    \begin{tabular}{lcccccc}
        \toprule
        \textbf{Metric} & AniTalker \cite{liu2024anitalker} & Ditto \cite{li2024ditto} & EchoMimic \cite{chen2025echomimic} & FLOAT \cite{ki2025float} & Hallo \cite{xu2024hallo} & \textbf{IMTalker (Ours)} \\
        \midrule
        Visual Quality & 3.62 $\pm$ 1.14 & 3.74 $\pm$ 1.08 & 3.86 $\pm$ 0.98 & 3.66 $\pm$ 1.24 & \underline{3.87 $\pm$ 1.08} & \textbf{4.06 $\pm$ 0.87} \\
        Audio-Lip Sync & 3.63 $\pm$ 1.24 & 3.39 $\pm$ 1.35 & 3.94 $\pm$ 0.85 & 3.95 $\pm$ 0.96 & \underline{3.99 $\pm$ 0.93} & \textbf{4.14 $\pm$ 0.83} \\
        Naturalness & 3.68 $\pm$ 1.06 & 3.62 $\pm$ 1.05 & \underline{4.03 $\pm$ 0.88} & 3.65 $\pm$ 1.00 & 3.88 $\pm$ 1.03 & \textbf{4.11 $\pm$ 0.80} \\
        \bottomrule
    \end{tabular}
\end{table*}
To comprehensively evaluate the perceptual quality of IMTalker, we conducted a user study with 30 participants, collecting 144 subjective responses across 48 generated videos. Our method was compared against five state-of-the-art baselines in two distinct settings: \textit{video-driven} and \textit{audio-driven}. Participants rated the results on a 5-point Likert scale (1=poor, 5=excellent) based on specific perceptual metrics.

For the \textbf{video-driven} setting, we assessed: (1) \textit{Visual Quality} (clarity and realism); (2) \textit{Motion Accuracy} (consistency of pose, expression, and gaze with the driving video); and (3) \textit{Identity Consistency} (preservation of source facial features). For the \textbf{audio-driven} setting, metrics included: (1) \textit{Visual Quality}; (2) \textit{Audio-Lip Synchronization} (alignment of lip motion with audio); and (3) \textit{Motion Naturalness} (diversity of head movement and vividness of expressions).

Quantitative results are presented in Tables~\ref{tab:user_study_video} and \ref{tab:user_study_audio}. As illustrated, IMTalker consistently outperforms all baselines across both settings. In the video-driven task, IMTalker achieves a remarkable score of \textbf{4.28} in \textit{Motion Accuracy}, demonstrating its superior capability in capturing fine-grained driving motions. Similarly, in the audio-driven task, our method leads with significantly higher scores in \textit{Audio-Lip Synchronization} (\textbf{4.14}) and \textit{Motion Naturalness} (\textbf{4.11}). Furthermore, the lower variance observed in IMTalker's ratings indicates a higher level of stability and consensus among users regarding the quality of our generated avatars.

% --- Tables Start ---

% ==========================================
% Section 5: Ablation
% ==========================================

% ==========================================
% Section 6: Demo
% ==========================================
\section{Qualitative Demonstrations} \label{sec:demos}

To provide a more intuitive assessment of the superiority and versatility of our method, we have included a comprehensive collection of video demonstrations alongside this supplementary material. These demos cover a wide range of scenarios, varying from diverse artistic styles to rigorous comparisons. Below, we detail the specific contents of each video category:

\begin{itemize}
    \item \textbf{Diverse Audio-Driven Generation:} We demonstrate the robustness and generalization capability of our model across various domains and languages. This category includes:
    \begin{itemize}
        \item \textit{Multilingual Speech:} High-fidelity lip-sync results in different languages, including English and Chinese.
        \item \textit{Cross-Domain Styles:} Generation results on out-of-domain samples such as artistic cartoons and stylized portraits, showing that our method is not limited to real-world human faces.
    \end{itemize}

    \item \textbf{Self- and Cross-Driven Reenactment:} We provide visualizations for two standard driving settings:
    \begin{itemize}
        \item \textit{Self-Reenactment:} Where the source identity is driven by their own motion, demonstrating the fidelity of reconstruction.
        \item \textit{Cross-Reenactment:} Where a source face is driven by the motion from a different identity, highlighting the model's ability in motion transfer.
    \end{itemize}

    \item \textbf{Audio-Driven Comparisons:} Comparisons with state-of-the-art audio-driven methods. These videos highlight our advantages in lip-synchronization accuracy, mouth shape detail, and overall image clarity.

    \item \textbf{Video-Driven Comparisons:} Comparisons with leading video-driven reenactment methods. These clips emphasize our method's superior performance in motion transfer and identity preservation.
    
    \item \textbf{Ablation Studies:} Visualizations demonstrating the impact of the Identity-Adaptive (IA) Module and the Hybrid Attention (HA) Strategy on generation quality and identity preservation.

    \item \textbf{Controllable Generation:} Demonstrations showing the capability to explicitly manipulate head pose and eye gaze directions independently of lip movements, offering flexible control for user-directed synthesis.

    \item \textbf{Long Video Generation:} A continuous long-sequence generation sample. This demonstrates the temporal stability of our method, proving that it maintains high fidelity and synchronization without drifting or accumulating artifacts over extended durations.
\end{itemize}

% ==========================================
% Section 7: Limitations
% ==========================================
\section{Limitations and Ethical Considerations} \label{sec:limitations}
\paragraph{Limitations}
Although IMTalker achieves efficient and vivid talking face generation, several limitations persist. First, the model performance degrades under extreme head rotations (e.g., yaw $>60^{\circ}$) or when significant new facial features appear (e.g., sticking out the tongue). To address this, we plan to incorporate multi-view datasets and richer facial expression data, such as \cite{kirschstein2023nersemble}, into our training process. Second, the model struggles with complex backgrounds, where disoccluded regions often exhibit blurry artifacts due to a lack of real-world physical priors. Integrating real-time video models like \cite{hacohen2024ltx} into the pipeline could effectively mitigate this issue. Finally, our current framework is restricted to fixed-resolution inputs and focuses solely on the facial region. Future work will introduce a ViT-based encoder to handle arbitrary input resolutions and incorporate full-body motion data to achieve efficient, high-fidelity full-body video generation.

\paragraph{Ethical Considerations} 
Our research aims to advance talking face generation by achieving real-time synthesis speeds under low computational resource constraints, making the technology viable for practical real-time scenarios. We acknowledge, however, that lowering the barrier to entry inevitably increases the potential risk of misuse, such as the creation of non-consensual deepfakes. To address these concerns, we advocate for responsible AI development, utilizing measures such as invisible watermarking for detection and enforcing strict license agreements against illegal usage. We believe that through proper safeguards and community self-regulation, the beneficial applications of this technology can be realized while effectively minimizing societal harm.
